# Supplementary material for: Simulation-guided Beam Search for Neural Combinatorial Optimization
Source: arXiv:2207.06190 source file (2022-11-17)
Supplement: Supplementary file 1 [file appendix_only_pdf_dummy.tex]

dummy line to adjust line numbers in the appendix\newline
dummy line to adjust line numbers in the appendix\newline
dummy line to adjust line numbers in the appendix\newline
dummy line to adjust line numbers in the appendix\newline
dummy line to adjust line numbers in the appendix\newline
dummy line to adjust line numbers in the appendix\newline
dummy line to adjust line numbers in the appendix\newline
dummy line to adjust line numbers in the appendix\newline
dummy line to adjust line numbers in the appendix\newline
dummy line to adjust line numbers in the appendix\newline
dummy line to adjust line numbers in the appendix\newline
dummy line to adjust line numbers in the appendix\newline
dummy line to adjust line numbers in the appendix\newline
dummy line to adjust line numbers in the appendix\newline
dummy line to adjust line numbers in the appendix\newline
dummy line to adjust line numbers in the appendix\newline
dummy line to adjust line numbers in the appendix\newline
dummy line to adjust line numbers in the appendix\newline
dummy line to adjust line numbers in the appendix\newline
dummy line to adjust line numbers in the appendix\newline
dummy line to adjust line numbers in the appendix\newline
dummy line to adjust line numbers in the appendix\newline
dummy line to adjust line numbers in the appendix\newline
dummy line to adjust line numbers in the appendix\newline
dummy line to adjust line numbers in the appendix\newline
dummy line to adjust line numbers in the appendix\newline
dummy line to adjust line numbers in the appendix\newline
dummy line to adjust line numbers in the appendix\newline
dummy line to adjust line numbers in the appendix\newline
dummy line to adjust line numbers in the appendix\newline
dummy line to adjust line numbers in the appendix\newline
dummy line to adjust line numbers in the appendix\newline
dummy line to adjust line numbers in the appendix\newline
dummy line to adjust line numbers in the appendix\newline
dummy line to adjust line numbers in the appendix\newline
dummy line to adjust line numbers in the appendix\newline
dummy line to adjust line numbers in the appendix\newline
dummy line to adjust line numbers in the appendix\newline
dummy line to adjust line numbers in the appendix\newline
dummy line to adjust line numbers in the appendix\newline
dummy line to adjust line numbers in the appendix\newline
dummy line to adjust line numbers in the appendix\newline
dummy line to adjust line numbers in the appendix\newline
dummy line to adjust line numbers in the appendix\newline
dummy line to adjust line numbers in the appendix\newline
dummy line to adjust line numbers in the appendix\newline
dummy line to adjust line numbers in the appendix\newline
dummy line to adjust line numbers in the appendix\newline
dummy line to adjust line numbers in the appendix\newline
dummy line to adjust line numbers in the appendix\newline
dummy line to adjust line numbers in the appendix\newline
dummy line to adjust line numbers in the appendix\newline
dummy line to adjust line numbers in the appendix\newline
dummy line to adjust line numbers in the appendix\newline
dummy line to adjust line numbers in the appendix\newline
dummy line to adjust line numbers in the appendix\newline
dummy line to adjust line numbers in the appendix\newline
dummy line to adjust line numbers in the appendix\newline
dummy line to adjust line numbers in the appendix\newline
dummy line to adjust line numbers in the appendix\newline
dummy line to adjust line numbers in the appendix\newline
dummy line to adjust line numbers in the appendix\newline
dummy line to adjust line numbers in the appendix\newline
dummy line to adjust line numbers in the appendix\newline
dummy line to adjust line numbers in the appendix\newline
dummy line to adjust line numbers in the appendix\newline
dummy line to adjust line numbers in the appendix\newline
dummy line to adjust line numbers in the appendix\newline
dummy line to adjust line numbers in the appendix\newline
dummy line to adjust line numbers in the appendix\newline
dummy line to adjust line numbers in the appendix\newline
dummy line to adjust line numbers in the appendix\newline
dummy line to adjust line numbers in the appendix\newline
dummy line to adjust line numbers in the appendix\newline
dummy line to adjust line numbers in the appendix\newline
dummy line to adjust line numbers in the appendix\newline
dummy line to adjust line numbers in the appendix\newline
dummy line to adjust line numbers in the appendix\newline
dummy line to adjust line numbers in the appendix\newline
dummy line to adjust line numbers in the appendix\newline
dummy line to adjust line numbers in the appendix\newline
dummy line to adjust line numbers in the appendix\newline
dummy line to adjust line numbers in the appendix\newline
dummy line to adjust line numbers in the appendix\newline
dummy line to adjust line numbers in the appendix\newline
dummy line to adjust line numbers in the appendix\newline
dummy line to adjust line numbers in the appendix\newline
dummy line to adjust line numbers in the appendix\newline
dummy line to adjust line numbers in the appendix\newline
dummy line to adjust line numbers in the appendix\newline
dummy line to adjust line numbers in the appendix\newline
dummy line to adjust line numbers in the appendix\newline
dummy line to adjust line numbers in the appendix\newline
dummy line to adjust line numbers in the appendix\newline
dummy line to adjust line numbers in the appendix\newline
dummy line to adjust line numbers in the appendix\newline
dummy line to adjust line numbers in the appendix\newline
dummy line to adjust line numbers in the appendix\newline
dummy line to adjust line numbers in the appendix\newline
dummy line to adjust line numbers in the appendix\newline
dummy line to adjust line numbers in the appendix\newline
dummy line to adjust line numbers in the appendix\newline
dummy line to adjust line numbers in the appendix\newline
dummy line to adjust line numbers in the appendix\newline
dummy line to adjust line numbers in the appendix\newline
dummy line to adjust line numbers in the appendix\newline
dummy line to adjust line numbers in the appendix\newline
dummy line to adjust line numbers in the appendix\newline
dummy line to adjust line numbers in the appendix\newline
dummy line to adjust line numbers in the appendix\newline
dummy line to adjust line numbers in the appendix\newline
dummy line to adjust line numbers in the appendix\newline
dummy line to adjust line numbers in the appendix\newline
dummy line to adjust line numbers in the appendix\newline
dummy line to adjust line numbers in the appendix\newline
dummy line to adjust line numbers in the appendix\newline
dummy line to adjust line numbers in the appendix\newline
dummy line to adjust line numbers in the appendix\newline
dummy line to adjust line numbers in the appendix\newline
