# Supplementary material for: Simulation-guided Beam Search for Neural Combinatorial Optimization
Source: arXiv:2207.06190 source file (2022-11-17)
Supplement: Supplementary file 2 [file SGBS_NeurIPS_appendix_v1.pdf]

## Appendix

### A Performance on real-world based instances

We further evaluate SGBS+EAS on nine real-world based instance sets from [15]. Each instance set consists of 20 instances that have similar characteristics (i.e., they have been sampled from the same underlying distribution). The instance sets differ significantly in terms of several structural properties, for example, the number of customers  $n$  and their position (e.g., clustered vs. random positions). A more detailed description of instance sets can be found in [15].

One major advantage of neural combinatorial optimization approaches over traditional handcrafted optimization methods is their ability to quickly learn customized heuristics for new problem settings. With the intention to evaluate the ability of SGBS+EAS to adapt towards different problem settings, we train a different model for each of the nine instance sets. This also makes sense in light of the fact that in real-world scenarios, the characteristics of instances usually do not change unexpectedly. We train each of the nine models using the POMO method [14] for 3,000 epochs (with 10,000 instances each).

The operations research literature has almost exclusively focused on solving instances sequentially, even though there are real-world scenarios in which a large number of instances need to be solved in parallel. Thus, to allow for a more fair comparison to established approaches, we solve instances sequentially and not in batches. We note that this is a slightly unfavorable setting for SGBS+EAS, which has been specifically designed to exploit the parallel computing capabilities of GPUs. To account for this new evaluation setting, we always perform 10 runs in parallel for EAS and SGBS+EAS. This improves the solution quality, while leading only to a slight increase of the required runtime.

We compare the performance of SGBS+EAS to only EAS, LKH3 [50], and HGS [45, 46]. For SGBS+EAS we set  $(\beta, \gamma) = (35, 5)$ , the learning rate  $\alpha = 0.005$  and  $\lambda = 0.05$ . We limit the search to 8 iterations of SGBS+EAS, and perform 30 EAS updates in each iteration (instead of only one EAS iteration as in previous experiments). We found that performing SGBS less often, but with higher  $\beta$  values improves the performance when solving instances sequentially because it better uses the available GPU memory. For EAS (without SGBS) we use identical values for  $\alpha$  and  $\lambda$  and we limit the runtime to the runtime of SGBS+EAS. For HGS and LKH3, we use the default parameters suggested by their developers. Note that we round the distances between customers to the nearest integer for all algorithms, as is common practice in the operations research literature. For each instance, we perform three independent runs per algorithm.

Table A shows the results. For HGS, we report the mean costs over all instances and runs. For EAS, SGBS+EAS, and LKH3 we report the absolute gap between their respective mean performance and the HGS mean. On all nine instance sets, SGBS+EAS significantly outperforms EAS. SGBS+EAS also finds solutions of higher quality than LKH3 for all nine instance sets, albeit while requiring

Table A: Performance for the CVRP on the XE instance sets from [15].

| Set   | $n$ | HGS Costs | Absolute gap to HGS mean |              |        | Avg. runtime in seconds |      |              |      |
|-------|-----|-----------|--------------------------|--------------|--------|-------------------------|------|--------------|------|
|       |     |           | EAS                      | SGBS<br>+EAS | LKH3   | HGS                     | EAS  | SGBS<br>+EAS | LKH3 |
| XE.1  | 100 | 30143.7   | +63.1                    | +27.1        | +641.4 | 22                      | 125  | 125          | 372  |
| XE.3  | 128 | 33435.9   | +93.5                    | +42.1        | +184.2 | 52                      | 178  | 178          | 122  |
| XE.5  | 180 | 26561.5   | +32.3                    | +17.4        | +42.9  | 44                      | 341  | 341          | 65   |
| XE.7  | 199 | 28608.5   | +142.7                   | +94.1        | +216.4 | 81                      | 400  | 400          | 215  |
| XE.9  | 213 | 11947.2   | +78.1                    | +42.3        | +131.4 | 82                      | 440  | 440          | 66   |
| XE.11 | 236 | 27487.1   | +266.2                   | +229.1       | +244.4 | 117                     | 556  | 556          | 67   |
| XE.13 | 269 | 33949.3   | +169.6                   | +139.0       | +572.3 | 103                     | 921  | 920          | 343  |
| XE.15 | 279 | 44597.8   | +353.6                   | +304.9       | +626.9 | 178                     | 870  | 869          | 347  |
| XE.17 | 297 | 36536.4   | +205.0                   | +161.0       | +495.5 | 126                     | 1118 | 1117         | 152  |

more time to do so. Overall, SGBS+EAS almost matches the solution quality of HGS with relative gaps between 0.07% (for XE\_5) to 0.83% (for XE\_11). This is an impressive achievement given that HGS is a highly specialized solver, relying on handcrafted heuristics that are the result of decades of research.

## B Implementation of greedy rollouts of SGBS

At each simulation phase of Algorithm 1, we perform  $\gamma$  greedy rollouts for each node contained in the set  $B$  (of size  $\beta$ ). Among those  $\gamma$  rollouts, one rollout is redundant, as it begins with the child node assigned with the largest probability. This rollout creates the same solution of one of nodes already examined in the previous simulation phase (unless we are at the root node). Therefore, in our implementation of SGBS, we improve the efficiency of our code by conducting only meaningful  $\gamma - 1$  rollouts. We skip the redundant rollout and simply reuse the result from the previous simulation. All in all, a total of  $\beta \times (\gamma - 1)$  new candidate solutions are examined at each simulation phase.

## C Search efficiency experiments in Section 3.3

The greedy method provides a single shot solution that represents the baseline quality of the policy network on a given problem instance. To improve the solution quality, each search method employs different tactics on how to make use of the information offered by the policy network (other than what its first choices are), as well as the evaluation results of the candidate solutions already produced. By limiting the total number of candidate solutions to the same value for all search methods, we aim to compare how effectively each search method utilizes all the information given to them.

Measurement of search efficiency in this way also reflects real-world application scenarios. While calculating the reward (or cost) of an arbitrary candidate solution is nearly instant for many benchmark CO problems used in the literature (*e.g.*, the TSP), many industry applications involve expensive reward functions  $\mathcal{R}$  (*e.g.*, if the task is optimization of training hyperparameters for a neural model, the reward is its measured performance *after* the training has been executed), making it the most expensive part throughout the whole optimization process. Thus, in such cases, it is more natural to seek the best performing search methods under the restriction on the allowed number of reward evaluations of candidate solutions.

**The number of candidate solutions allowed** For experiments based on the CVRP instances with  $n = 100$  (Figures 2 (a) and (c)), the number of candidate solutions allowed is 1.2K. For CVRP experiments with  $n = 200$  instances (Figure 2 (b)), this number is limited to 2.4K. These limits are chosen to match the estimated total number of greedy rollouts simulated by the SGBS method when its hyperparameters  $(\beta, \gamma)$  are set to  $(4, 4)$ .

This estimation works as follows. As explained in Section B, SGBS with  $\beta = 4$ , and  $\gamma = 4$  makes at most  $\beta \times (\gamma - 1) = 12$  new candidate solutions (greedy rollouts) at each simulation phase. A simulation phase is needed whenever it adds a customer node to a partially completed solution, which happens 100 (200) times for  $n = 100$  (200). This results in 1.2K (2.4K) total greedy rollouts for each problem instance. This is actually a slightly overestimated value, because SGBS sometimes runs less than 12 rollouts during a simulation phase. This happens when there are only a few unvisited customer nodes left towards the end of the search, or when the load on the vehicle limits the number of valid next customer nodes available.

**Search details** The sampling, active search and EAS methods can repeat the search process freely and produce as many candidate solutions as desired. Thus, we re-apply these search methods until enough candidate solutions are collected. Beam Search and MCTS, on the other hand, cannot simply be repeated. Beam Search is explicitly given a beam width of 1.2K (2.4K) from the beginning of the search, which then creates that number of complete solutions all at once. MCTS runs 12 greedy simulations at each depth level in the search tree, similar to SGBS. Our implementation of MCTS is

552 similar to that of Xing *et al.* [33] but with their Eq.(8) changed to

$$U(s, a) = c_{\text{puct}} P(s, a) \frac{\sqrt{\sum_b N(s, b)}}{0.1 + N(s, a)}. \quad (\text{C.1})$$

553 Here,  $N(s, a)$  is the visit count from a node  $s$  to its child  $a$ . The value of  $U(s, a)$  decreases as more  
554 visits are made to  $a$ , and this encourages exploration within the MCTS algorithm. ( $c_{\text{puct}}$  is some  
555 constant, and  $P(s, a)$  is the prior probability for choosing  $a$ .) The constant 0.1 in the denominator  
556 has been changed from 1 to improve the performance of MCTS. This change induces reasonable  
557 exploration within the 12-simulation-limit, which is much less than the usual number of simulations  
558 ( $> 100$ ) expected by the original MCTS algorithm. Finally, we do not use the  $\times 8$  instance augmen-  
559 tation technique [14] on any of the search methods being compared in this experiment, as it will  
560 increase the number of the produced candidate solutions by a factor of 8.

561 **Adjustments made for POMO-trained policy network** We use the policy neural network that is  
562 trained with RL by the POMO method [14]. The high performance of the POMO training method  
563 on the CVRP relies on the diversification of the candidate solutions induced by its manual (user-  
564 designated) selection of the first nodes. While this POMO approach leads to a significant improve-  
565 ment in the quality of the trained model, it results in the policy network never being properly trained  
566 for making good suggestions for the first node. This causes a complication for our search efficiency  
567 experiment, as our search methods are not provided with a proper policy for what to choose for the  
568 first customer nodes.

569 For the greedy results used as the baselines in Figure 2, we actually make 100 (200) different greedy  
570 solutions starting from each node, and sort them based on their performance. We use the best one  
571 to represent the greedy method. Note that this is how the inference is done in the original POMO  
572 paper. For the other search methods, however, we do not repeat the search 100 (200) times like this,  
573 as this would mean that, for example, the sampling method only gets to create 12 candidate solutions  
574 per starting node. This is wasteful, as most of the nodes are unfit to be used as the starting node.  
575 Instead, we choose  $\beta = 4$  nodes as the “official” first node candidates, based on the greedy rollout  
576 results. Note that all of them are likely to be the optimal choices for starting the CVRP solution. For  
577 the sampling, active search, and EAS methods, we generate 0.3K (0.6K) candidate solutions starting  
578 from each of these four nodes. For the beam search and SGBS, we use these four nodes as the initial  
579 beam front and have the search tree expand from there. For MCTS, we simply choose just one node,  
580 which is the best out of the four, as the starting node and the MCTS method expands from there.

## 581 D Different sets of $(\beta, \gamma)$ for SGBS

582 Figure D shows the runtime and the performance of the SGBS algorithm with different values for  $\beta$   
583 and  $\gamma$  on the test set [4] of 10,000 CVRP instances with  $n = 100$ . The performance gap drops sharply

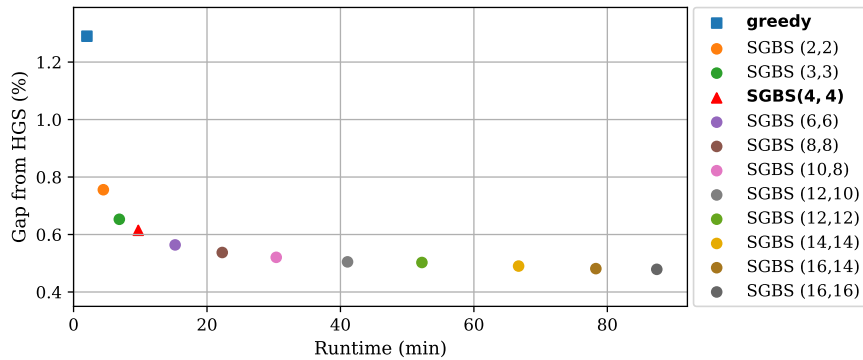

Figure D: SGBS results on the CVRP with  $n = 100$ , with different choices for parameters  $(\beta, \gamma)$ .

584 from the greedy result as the SGBS algorithm is applied, and, with larger  $\beta$  and  $\gamma$ , higher quality  
585 solutions are achieved. However, the performance gain quickly becomes marginal. Table 1 in the  
586 main text contains the result of  $(\beta, \gamma) = (4, 4)$ .

## 587 E Different sets of $(\beta, \gamma)$ for SGBS+EAS

588 Using a small set of instances, the performance of SGBS+EAS can be examined over different  
589 choices of  $\beta$  and  $\gamma$  in a relatively short time. In Figure E, we find that  $(\beta, \gamma) = (4, 4)$  gives the best  
590 result for the CVRP with 100 nodes. However, as long as the values for  $\beta$  and  $\gamma$  are not chosen  
591 too small or too large, the search algorithm consistently finds decent solutions. Within the range of  
592  $[2, 12]$  for both  $\beta$  and  $\gamma$ , SGBS+EAS displays less than 0.15% gaps from the HGS solution.

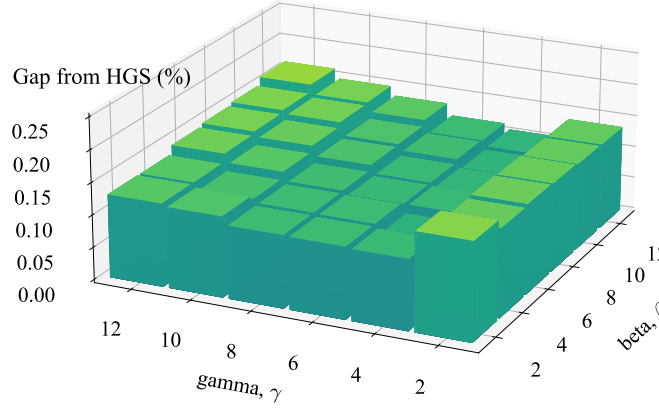

Figure E: The quality of incumbent solutions after 3-hour runs of SGBS+EAS with different values for parameters  $\beta$  and  $\gamma$ , on 1,000 instances of the CVRP with  $n = 100$ .

## 593 F TSP & CVRP experiments

594 **Baselines** We run all the baseline algorithms ourselves and compare their results and runtimes  
595 based on the identical test sets in Table 1. Note that most neural baseline approaches are not ex-  
596 plicitly designed for the generalization tests we conduct. Also, for each search method we simply  
597 re-use the hyperparameters optimized for  $n = 100$  problems across all problem sizes, and therefore  
598 some generalization test results may improve substantially with appropriate adjustments to the hy-  
599 perparameters. As for the DACT results on the TSP generalization tests, we opt to report no values  
600 in Table 1 as the results are not that satisfying.

601 **POMO model** For our SGBS+EAS experiments and the ablation tests, we use the neural policy  
602 networks trained by the POMO method [14] ourselves. Models are regularly saved during training,  
603 and we select intermediate models that have not fully converged (*i.e.*, early stop, see Appendix I)  
604 for our experiments. The model we choose for TSP100 experiments is trained for 1900 epochs (10  
605 days) and for CVRP100 experiments the model is trained for 10,000 epochs (8 days).

## 606 G FFSP experiments

607 **Baselines** CPLEX, Genetic Algorithm (GA), and Particle Swarm Optimization (PSO) results are  
608 adopted from the MatNet paper [13]. The authors have provided us the raw data so that we can  
609 display more digits for the baseline results in Table 2. The original MaNet paper reports runtimes  
610 of single-thread processes after dividing them by 8 (as an attempt to provide a more balanced view  
611 between the runtimes of CPU- and GPU-based methods). Our paper, however, uses the wall-clock  
612 time convention, so the runtimes of GA and PSO in Table 2 have been adjusted accordingly.

**MatNet model training** For the SGBS(+EAS) experiments and the related ablation tests on the FFSP, we use MatNet architecture [13] for the policy neural network. To solve the FFSP with job count  $n=20, 50$  and  $100$ , we train the MatNet model for 54, 95, 120 epochs (2 hours, 5 hours, 35 hours), respectively. We build and train the models based on the MatNet codes shared on the public repository, using the default hyperparameters.

**Instance augmentation** MatNet allows different instance augmentation technique than what is used for the routing problems. By shuffling the order of the one-hot vector sequence fed to the MatNet during the initialization, one can effectively achieve different augmentations for the given FFSP instance. Hence, for the FFSP, one can freely choose any large number as the augmentation factor. In the MatNet paper, the  $\times 128$  instance augmentation is used as the default setting.

While the  $\times 128$  augmentation is a reasonable choice for the greedy inference, it is too much for SGBS(+EAS) algorithm. For better time efficiency, we use the  $\times 8$  instance augmentation for all the MatNet-based search methods compared on Table 2, except for the greedy result. More specifically, we first run the greedy search using the  $\times 128$  instance augmentation. Based on this result, we select the best 8 instance augmentations and use these 8 for all the other MatNet-based methods we test.

## H Short pre-tain

In Figure H, solutions found by the greedy and SGBS+EAS methods are compared to those of LKH3. A test set of 1,000 instances of CVRP with  $n=100$  is used, and SGBS+EAS is run for 3 hours. (This is equivalent to 30-hour run of SGBS+EAS on 10K problem instances demonstrated in Table 1.) We find that the models with only 2-hour pre-train or more can produce solutions of higher quality than those of the LKH3.

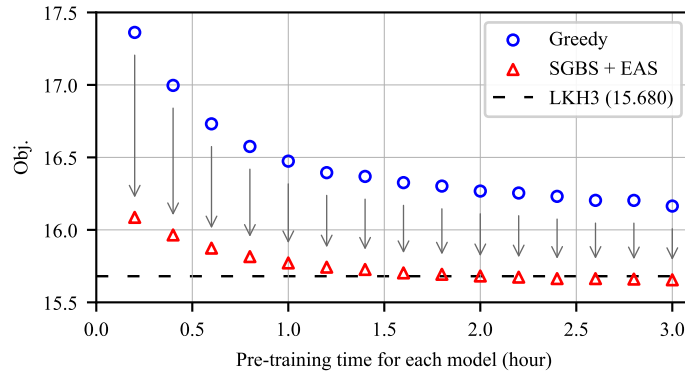

Figure H: Mean cost of the CVRP with  $n=100$  solutions produced based on different neural models, before (blue circle) and after (red triangle) applying the SGBS+EAS algorithm. Here, each model is pre-trained only for a very short time ( $\leq 3$  hours) in different durations.

## I Early stops and entropy regulation

Shown in Figure I (a) is the mean cost of greedy solutions to the CVRP with  $n=100$ , generated from a neural model trained by the POMO method. The quality of the policy network, measured by the performance of its greedy solutions, continues to improve with longer (pre-)training. While not shown in the figure, the training curve never converges completely even after 1,000 hours of training. Hence, in order to prepare a policy network to its highest quality, one is forced to wait many weeks before stopping the training.

To our surprise, however, when we use the SGBS+EAS algorithm at test time, it is found that such extended pre-training of the policy neural network actually degrades the solution quality. Red trian-

gles in Figure I (b) are the mean cost of the incumbent solutions found by 3-hour run of SGBS+EAS. It is observed that pre-training longer than 200 hours does not help improve the solution quality, and in fact, the longer the training the worse results are returned (a positive slope of the red line). In a sense, these models are “over-fitted” to the distribution of the training instances, which make it more difficult to fine-tune the models to a single, specific target instance.

In order to alleviate this over-fitting problem, we try regulating the entropy of the model during the training. The policy gradient  $\nabla_{\theta} J$  used by the POMO training method is described in Eq.(3) of [14], which we modify by adding the entropy regulation as

$$\nabla_{\theta} J' = \nabla_{\theta} J + \lambda_1 \frac{1}{N} \sum_{i=1}^N \sum_{t=2}^M \nabla_{\theta} \mathcal{H}(p_{\theta}(\cdot | s, a_{1:t-1}^i)). \quad (\text{I.1})$$

Here,  $\mathcal{H}$  is the entropy function. Note that the notations used in this equation follows those defined in [14], and they are slightly different from the notations used in our paper (*e.g.*, the meaning of  $N$ , etc.). By using a positive value for  $\lambda_1$ , we can increase the entropy on the output of the model. Blue squares in Figure I (b) show that this entropy regulation scheme works, and we can prevent (or at least mitigate) the over-fitting problem at the pre-training stage.

We can further improve the search performance by incorporating the entropy regulation into the SGBS+EAS algorithm as well, by replacing  $\nabla_{\psi} J_{RL}$  in line 8 of Algorithm 2 with

$$\nabla_{\psi} J'_{RL} = \nabla_{\psi} J_{RL} + \lambda_2 \frac{1}{M} \sum_{i=1}^M \sum_{d=0}^{N-1} \nabla_{\psi} \mathcal{H}(\tilde{\pi}_{\theta, \psi}(\cdot | s_d^i)). \quad (\text{I.2})$$

Green diamond markers in Figure I (b) show that if the value of  $\lambda_2$  is well-tuned, the quality of the incumbent solutions found by SGBS+EAS can be boosted a little further.

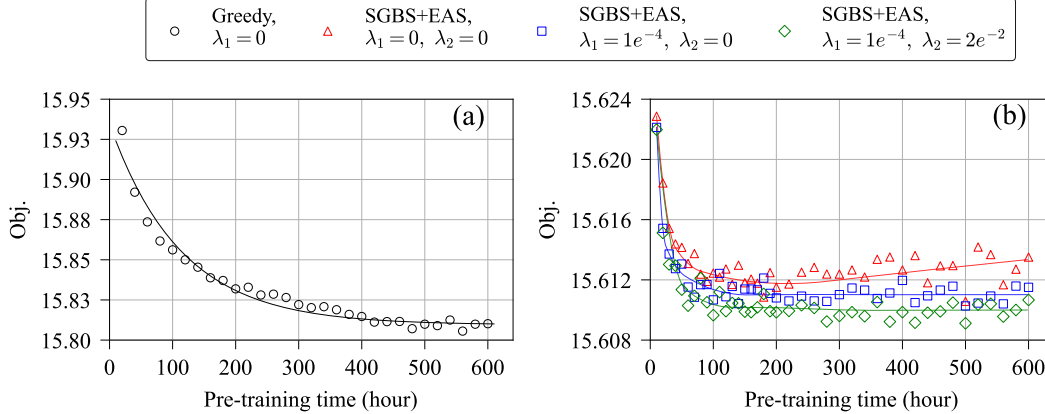

Figure I: The mean cost of the CVRP with  $n = 100$  solutions found by different search methods on various models. A test set consisting of 1,000 problem instances is used. (a) shows the greedy results, and (b) shows three SGBS+EAS results with different  $\lambda_1$  and  $\lambda_2$  (explained in the text) after 3-hour search processes. Each data point represents a different model, pre-trained in varying degrees. Lines are drawn to guide the eye only.

## References

- [1] André Hottung, Yeong-Dae Kwon, and Kevin Tierney. Efficient active search for combinatorial optimization problems. *International Conference on Learning Representations*, 2022.
- [2] Yoshua Bengio, Andrea Lodi, and Antoine Prouvost. Machine learning for combinatorial optimization: a methodological tour d’ horizon. *European Journal of Operational Research*, 2020.
- [3] Irwan Bello, Hieu Pham, Quoc V. Le, Mohammad Norouzi, and Samy Bengio. Neural combinatorial optimization with reinforcement learning. *ICLR (Workshop)*, 2017.
- [4] Wouter Kool, Herke van Hoof, and Max Welling. Attention, learn to solve routing problems! *International Conference on Learning Representations*, 2019.
- [5] Levente Kocsis and Csaba Szepesvári. Bandit based monte-carlo planning. In *Machine Learning: ECML 2006*, pages 282–293, Berlin, Heidelberg, 2006. Springer Berlin Heidelberg.
- [6] Rémi Coulom. Efficient selectivity and backup operators in monte-carlo tree search. In *Computers and Games*, pages 72–83, Berlin, Heidelberg, 2007. Springer Berlin Heidelberg.
- [7] Oriol Vinyals, Meire Fortunato, and Navdeep Jaitly. Pointer networks. *Advances in Neural Information Processing Systems* 28, 2015.
- [8] Mohammadreza Nazari, Afshin Oroojlooy, Lawrence Snyder, and Martin Takac. Reinforcement learning for solving the vehicle routing problem. *Advances in Neural Information Processing Systems* 31, 2018.
- [9] Wouter Kool, Herke van Hoof, Joaquim Gromicho, and Max Welling. Deep policy dynamic programming for vehicle routing problems. *arXiv preprint arXiv:2102.11756*, 2021.
- [10] Chaitanya K Joshi, Quentin Cappart, Louis-Martin Rousseau, and Thomas Laurent. Learning the traveling salesperson problem requires rethinking generalization. *Constraints*, pages 1–29, 2022.
- [11] Elias Khalil, Hanjun Dai, Yuyu Zhang, Bistra Dilkina, and Le Song. Learning combinatorial optimization algorithms over graphs. *Advances in Neural Information Processing Systems* 30, 2017.
- [12] Michel Deudon, Pierre Cournut, Alexandre Lacoste, Yossiri Adulyasak, and Louis-Martin Rousseau. Learning heuristics for the TSP by policy gradient. In *International Conference on the Integration of Constraint Programming, Artificial Intelligence, and Operations Research*, pages 170–181. Springer, 2018.
- [13] Yeong-Dae Kwon, Jinho Choo, Iljoo Yoon, Minah Park, Duwon Park, and Youngjune Gwon. Matrix encoding networks for neural combinatorial optimization. *Advances in Neural Information Processing Systems* 34, 2021.
- [14] Yeong-Dae Kwon, Jinho Choo, Byoungjip Kim, Iljoo Yoon, Youngjune Gwon, and Seungjai Min. Pomo: Policy optimization with multiple optima for reinforcement learning. *Advances in Neural Information Processing Systems* 33, 2020.
- [15] André Hottung and Kevin Tierney. Neural large neighborhood search for the capacitated vehicle routing problem. *European Conference on Artificial Intelligence*, pages 443–450, 2020.
- [16] Xinyun Chen and Yuandong Tian. Learning to perform local rewriting for combinatorial optimization. *Advances in Neural Information Processing Systems* 32, 2019.
- [17] Paulo R. de O. da Costa, Jason Rhuggenaath, Yingqian Zhang, and Alp Akcay. Learning 2-opt heuristics for the traveling salesman problem via deep reinforcement learning. *ACML*, pages 465–480, 2020.
- [18] Yaoxin Wu, Wen Song, Zhiguang Cao, Jie Zhang, and Andrew Lim. Learning improvement heuristics for solving routing problems. *IEEE Transactions on Neural Networks*, 2021.
- [19] Yining Ma, Jingwen Li, Zhiguang Cao, Wen Song, Le Zhang, Zhenghua Chen, and Jing Tang. Learning to iteratively solve routing problems with dual-aspect collaborative transformer. *Advances in Neural Information Processing Systems* 34, pages 11096–11107, 2021.
- [20] Minsu Kim, Jinkyoo Park, and Joungho Kim. Learning collaborative policies to solve np-hard routing problems. *Advances in Neural Information Processing Systems* 34, pages 10418–10430, 2021.
- [21] Sirui Li, Zhongxia Yan, and Cathy Wu. Learning to delegate for large-scale vehicle routing. *Advances in Neural Information Processing Systems* 34, 2021.

- [22] Liang Xin, Wen Song, Zhiguang Cao, and Jie Zhang. Neurolkh: Combining deep learning model with lin-kernighan-helsgaun heuristic for solving the traveling salesman problem. *Advances in Neural Information Processing Systems 34*, 2021.
- [23] Arthur Delarue, Ross Anderson, and Christian Tjandraatmadja. Reinforcement learning with combinatorial actions: An application to vehicle routing. *Advances in Neural Information Processing Systems 33*, pages 609–620, 2020.
- [24] Liang Xin, Wen Song, Zhiguang Cao, and Jie Zhang. Multi-decoder attention model with embedding glimpse for solving vehicle routing problems. In *Proceedings of the AAAI Conference on Artificial Intelligence*, volume 35, pages 12042–12049, 2021.
- [25] Yining Ma, Jingwen Li, Zhiguang Cao, Wen Song, Hongliang Guo, Yuejiao Gong, and Yeow Meng Chee. Efficient neural neighborhood search for pickup and delivery problems. *arXiv preprint arXiv:2204.11399*, 2022.
- [26] Chun-Cheng Lin, Der-Jiunn Deng, Yen-Ling Chih, and Hsin-Ting Chiu. Smart manufacturing scheduling with edge computing using multiclass deep q network. *IEEE Transactions on Industrial Informatics*, 15(7):4276–4284, 2019.
- [27] Cong Zhang, Wen Song, Zhiguang Cao, Jie Zhang, Puay Siew Tan, and Xu Chi. Learning to dispatch for job shop scheduling via deep reinforcement learning. *Advances in Neural Information Processing Systems 33*, pages 1621–1632, 2020.
- [28] Emre Yolcu and Barnabás Póczos. Learning local search heuristics for boolean satisfiability. *Advances in Neural Information Processing Systems 32*, 2019.
- [29] Vitaly Kurin, Saad Godil, Shimon Whiteson, and Bryan Catanzaro. Can q-learning with graph networks learn a generalizable branching heuristic for a sat solver? *Advances in Neural Information Processing Systems 33*, pages 9608–9621, 2020.
- [30] Ruoyu Cheng and Junchi Yan. On joint learning for solving placement and routing in chip design. *Advances in Neural Information Processing Systems 34*, 2021.
- [31] Azalia Mirhoseini, Anna Goldie, Mustafa Yazgan, Joe Wenjie Jiang, Ebrahim Songhori, Shen Wang, Young-Joon Lee, Eric Johnson, Omkar Pathak, Azade Nazi, et al. A graph placement methodology for fast chip design. *Nature*, 594(7862):207–212, 2021.
- [32] Chaitanya K Joshi, Thomas Laurent, and Xavier Bresson. An efficient graph convolutional network technique for the travelling salesman problem. *INFORMS Annual Meeting 2019, Session on Boosting Combinatorial Optimization using Machine Learning*.
- [33] Zhihao Xing and Shikui Tu. A graph neural network assisted monte carlo tree search approach to traveling salesman problem. *IEEE Access*, 8:108418–108428, 2020.
- [34] Zhang-Hua Fu, Kai-Bin Qiu, and Hongyuan Zha. Generalize a small pre-trained model to arbitrarily large tsp instances. In *Proceedings of the AAAI Conference on Artificial Intelligence*, volume 35, pages 7474–7482, 2021.
- [35] David Silver, Aja Huang, Chris J. Maddison, Arthur Guez, Laurent Sifre, George van den Driessche, Julian Schrittwieser, Ioannis Antonoglou, Veda Panneershelvam, Marc Lanctot, Sander Dieleman, Dominik Grewe, John Nham, Nal Kalchbrenner, Ilya Sutskever, Timothy Lillicrap, Madeleine Leach, Koray Kavukcuoglu, Thore Graepel, and Demis Hassabis. Mastering the game of go with deep neural networks and tree search. *Nature*, 529(7587):484–489, Jan 2016.
- [36] Renato Negrinho, Matthew Gormley, and Geoffrey J Gordon. Learning beam search policies via imitation learning. *Advances in Neural Information Processing Systems 31*, 2018.
- [37] Marc Huber and Günther R Raidl. Learning beam search: Utilizing machine learning to guide beam search for solving combinatorial optimization problems. In *International Conference on Machine Learning, Optimization, and Data Science*, pages 283–298. Springer, 2021.
- [38] Kenshin Abe, Zijian Xu, Issei Sato, and Masashi Sugiyama. Solving np-hard problems on graphs with extended alphago zero. *arXiv preprint arXiv:1905.11623*, 2019.
- [39] Elias Khalil, Pierre Le Bodic, Le Song, George Nemhauser, and Bistra Dilkina. Learning to branch in mixed integer programming. In *Proceedings of the AAAI Conference on Artificial Intelligence*, volume 30, 2016.



- 758 [40] André Hottung, Shunji Tanaka, and Kevin Tierney. Deep learning assisted heuristic tree search for the  
759 container pre-marshalling problem. *Computers & Operations Research*, 113:104781, 2020.
- 760 [41] Tristan Cazenave. Monte carlo beam search. *IEEE Transactions on Computational Intelligence and AI in*  
761 *games*, 4(1):68–72, 2012.
- 762 [42] Hendrik Baier and Mark HM Winands. Beam monte-carlo tree search. In *2012 IEEE Conference on*  
763 *Computational Intelligence and Games (CIG)*, pages 227–233. IEEE, 2012.
- 764 [43] Jorik Jooken, Pieter Leyman, Patrick De Causmaecker, and Tony Wauters. Exploring search space trees  
765 using an adapted version of monte carlo tree search for combinatorial optimization problems. *arXiv*  
766 *preprint arXiv:2010.11523*, 2020.
- 767 [44] Stefan Edelkamp, Max Gath, Tristan Cazenave, and Fabien Teytaud. Algorithm and knowledge engi-  
768 neering for the tsptw problem. In *2013 IEEE Symposium on Computational Intelligence in Scheduling*  
769 *(CISched)*, pages 44–51. IEEE, 2013.
- 770 [45] Thibaut Vidal, Teodor Gabriel Crainic, Michel Gendreau, Nadia Lahrichi, and Walter Rei. A hybrid  
771 genetic algorithm for multidepot and periodic vehicle routing problems. *Operations Research*, 60(3):611–  
772 624, 2012.
- 773 [46] Thibaut Vidal. Hybrid genetic search for the cvrp: Open-source implementation and swap\* neighborhood.  
774 *Computers & Operations Research*, 140:105643, 2022.
- 775 [47] Chuan Guo, Geoff Pleiss, Yu Sun, and Kilian Q. Weinberger. On calibration of modern neural networks.  
776 In *Proceedings of the 34th International Conference on Machine Learning*, volume 70, 2017.
- 777 [48] David L Applegate, Robert E Bixby, Vasek Chvatal, and William J Cook. *The traveling salesman problem:*  
778 *a computational study*. Princeton university press, 2006.
- 779 [49] IBM ILOG CPLEX Optimization Studio. V20.1: User’s Manual for CPLEX. *IBM Corp*, 2020.
- 780 [50] Keld Helsgaun. *An Extension of the Lin-Kernighan-Helsgaun TSP Solver for Constrained Traveling*  
781 *Salesman and Vehicle Routing Problems: Technical report*. Roskilde Universitet, December 2017.
